# Supplementary material for: Bethe-Heitler type radiative corrections to deeply virtual neutrinoproduction of mesons
Source: arXiv:1301.7014 ancillary file (2013-03-10)
Supplement: Supplementary file 1 [file README.pdf]

## Code for evaluation of BH corrections to the $\nu$ DVMP cross-sections

This package provides a library `libDVMP` which may be used for evaluation of the  $\nu$ DVMP cross-sections and electromagnetic Bethe-Heitler corrections with various GPD models. Below are given short instructions how to compile and use it.

**Description:** This package provides a library `libDVMP` which may be used for evaluation of the  $\nu$ DVMP cross-sections and electromagnetic Bethe-Heitler corrections in the framework discussed in the paper. The common header file ‘`headers/NuDVMP.h`’ includes all the necessary definitions.

To evaluate the contributions of DVMP, Bethe-Heitler (BH) and interference term, You should call functions

```
double dvmp_XSection_dlnx_dt_dQ2_dphi(AbstractGPD
    fun, double phi, double* kins, process
    p);
double BH_XSection_dlnx_dt_dQ2_dphi(AbstractGPD
    fun, double phi, double* kins, process
    p, Harmonics* Hcs)
and
double intf_XSection_dlnx_dt_dQ2_dphi(AbstractGPD
    fun, double phi, double* kins, process
    p, Harmonics* Hcs)
```

respectively. Upon successful completion, the value of the corresponding cross-section  $x_B d^4\sigma/dt dx_B dQ^2 d\phi$  for a given angle  $\phi$  is returned. In case of the DVMP cross-section, the value of the angle  $\phi$  is ignored since the cross-section doesn’t depend on it. For BH and interference terms, structure `Harmonics` has elements `c[n]` and `s[n]` which correspond to the cosine and sine harmonics of the corresponding cross-section. The first argument `fun` in all three functions corresponds to an external GPD function declared in `headers/GPDPDF.h`, the array `kins` contains kinematic variables ordered as `kins[]={y, xB, t, Q}`, where  $y = p \cdot q / p \cdot k$ ,  $x_B$  is a Bjorken variable,  $t$  is the momentum transfer squared,  $t = \Delta^2$ ,  $Q = \sqrt{-q^2}$ . The structure `process p` declared in `headers/phys.h` contains information on particles participating in the process and has the following elements:

|                            |                                                                                        |
|----------------------------|----------------------------------------------------------------------------------------|
| <code>p.projectile</code>  | initial lepton ( $\nu/\bar{\nu}$ )                                                     |
| <code>p.target</code>      | target ( $p/n$ )                                                                       |
| <code>p.finalMeson</code>  | produced meson from octet of pseudogolstones ( $\pi^{0,\pm}, K^{L,S}, K^{\pm}, \eta$ ) |
| <code>p.finalBaryon</code> | produced baryon from lowest octet ( $p, n, \Lambda, \Sigma^{0,\pm}$ )                  |
| <code>p.finalLepton</code> | produced lepton ( $\nu, \bar{\nu}, \mu^{\pm}$ )                                        |

The GPD models needed for numerical evaluations are placed in separate library files in folder `libraries/`. With this package, we provide the Kroll-Goloskokov [1, 2] GPD model (file `libKrollGoloskokovGPD.so`) and a simple zero skewness GPD model (`libZeroSkewness.so`) described in the text of the paper.

**Prerequisites:** To compile this code, You need to have C compiler, `make` utility and a GNU scientific library (GSL) installed. The code was tested with `gcc` v. 4.4 and 4.6 on Linux x86-64 platform.

**Compilation:** To compile the code, You have to run `make` all in the code main directory. This will build the two above-mentioned GPD libraries, the  $\nu$ DVMP library (`libDVMP.so`, `libDVMP.a`) and an example driving application `NuDVMP_Q2` (see `src/DVMP_Q2.c`) which shows how to load GPDs from corresponding libraries and evaluates the cross-section as a function of  $Q^2$ .

**Running:** After compilation, run from command-line

```
./NuDVMP_Q2 --NeutrinoType NuMu --Target
Proton --Lepton MuMinus --Meson PiPlus
--Baryon Proton --lepton-fraction 0.25
--xBj 0.1 --DeltaTr 0.2 --gpd-model
libraries/libKrollGoloskokovGPD.so
```

or in a brief form

```
./NuDVMP_Q2 -N NuMu -T Proton -L MuMinus
-M PiPlus -B Proton -y 0.25 -x 0.1 -d 0.2
-g libraries/libKrollGoloskokovGPD.so
```

(optionally, instead of particle names, You can use their PDG codes; only particles and processes mentioned in the text of the paper are supported). This will evaluate and print the cosine and sine harmonics  $c_n, s_n$  defined in Eq. (29) of the main paper, for the process  $\nu p \rightarrow \mu^- \pi^+ p$  as a function of  $Q^2$  at  $y = 0.25$ ,  $\Delta_{\perp} = 0.2$ ,  $x_B = 0.1$  with Kroll-Goloskokov GPD model.

**Adding new GPD models:** In order to add a new GPD model, You have to implement the function `ExternalGPD(double x, struct GPDKins k)`, where `x` is the quark light-cone fraction and `struct GPDKins` declared in `headers/GPDPDF.h` keeps all the information on the target kinematics and has the following elements:

|                         |                                                                                                                    |
|-------------------------|--------------------------------------------------------------------------------------------------------------------|
| <code>k.xi</code>       | skewness parameter $\xi$                                                                                           |
| <code>k.t</code>        | momentum transfer $t = \Delta^2$                                                                                   |
| <code>k.Q</code>        | Scale at which GPD is taken                                                                                        |
| <code>k.flavour</code>  | GPD flavor                                                                                                         |
| <code>k.GPD_type</code> | Type of GPD, can be <code>GPD_H</code> ,<br><code>GPD_E</code> , <code>GPD_HTilde</code> , <code>GPD_ETilde</code> |

After compilation of the file `libNewGPD.so`, You may try to

generate the cross-section using `--gpd-model` option discussed above.

For more details, please see the header files in `headers/` directory. Each function has a Doxygen-style comments with detailed description. Corresponding `.c`-files are in `src/` directory.

---

[1] S. V. Goloskokov and P. Kroll, Eur. Phys. J. C **50**, 829 (2007) [hep-ph/0611290].

[2] S. V. Goloskokov and P. Kroll, Eur. Phys. J. C **53**, 367 (2008) [arXiv:0708.3569 [hep-ph]].
